# Supplementary material for: Bayesian model calibration for block copolymer self-assembly: Likelihood-free inference and expected information gain computation via measure transport
Source: arXiv:2206.11343 source file (2022-06-22)
Supplement: Supplementary file 1 [file sec_03.tex]

\section{Numerical construction of prior admissable set}
\label{app:prior_construction_details}

To produce the numerical ODT curves, we found minimizers $\state^i = \mathcal{F}(\x^i, \z^i) \in \mathcal{S}^{\textrm{OK}}(\x^i)$, for sparsely populated grid points in parameter space, where for $\x^i = (m^i, \epsilon^i, \sigma^i)$, we considered parameters $m^i\in (0, 1/\sqrt{3})$, $\epsilon^i \in (0, 1.5)$, and $\sigma^i \in (0, 5)$. If $\|\state^i - \overline{\state}^i\|_{L^2(\mathcal{D})} > 1e^{-8}$, we consider the parameter $\x^i$ as admissible, given the hypothesis that $\overline{\state}^i := m^i$ is not the global minimizer of $\mathcal{E}_{\x^i}^{\textrm{OK}}$~\cite{}. We then refined the sampling of parameter space until a boundary was clearly observed, separating admissible and inadmissible parameters.  

\begin{itemize}
    \item $\epsilon \in (\epsilon_{\textrm{min}}, \epsilon_{\textrm{max}}^m)$
    \item $\sigma_{\textrm{min}}^m(\epsilon) = a_{\textnormal{min}}(m ) \exp(-b_{\textnormal{min}}(m )\epsilon)$
    \item $\sigma_{\textrm{max}}^m(\epsilon)= a_{\textnormal{max}}(m ) \exp(-b_{\textnormal{max}}(m ) \epsilon)$
\end{itemize}

\textbf{place the actual equation for the regression coefficients for the polynomials, as well as a table of the coefficeints for  m, for a and b here }

Given the admissible set $\mathcal{A}$ for the uniform prior density $\pi_{\bx}$ in \eqref{eq:admissible_set_uniform_prior}, we describe a triangular transport map $S^{\bx}$ that pushes forward $\pi_{\bx}$ to a standard uniform $\mathcal{U}(0,\identity_3)$ by describing a triangular bijection between $\mathcal{A}$ and the unit cube $(0,10^3)$. 
\begin{equation}
    S^{\bx}(\x) = \begin{bmatrix*}[l]S^{m}(m), \\ S^{\epsilon}(m,\epsilon)\\S^{\sigma}(m,\epsilon,\sigma) \end{bmatrix*},
\end{equation}
where $S^{m}: (0, 1/\sqrt{3}) \to (0,1)$, $S^{\epsilon}(m,\cdot): (\epsilon_{\textrm{min}},\epsilon_{\textrm{max}}^m) \to (0,1)$,
$S^{\sigma}(m,\epsilon,\cdot):(\sigma_{\textrm{min}}^m(\epsilon)$,$\sigma_{\textrm{max}}^m(\epsilon)) \to (0,1)$, and
\begin{align}\begin{split}S^{m}(m)&= \sqrt{3}m,\\
S^{\epsilon}(m,\epsilon) &= \frac{\int_{\epsilon_{\textrm{min}}}^{\epsilon}\sigma_{\textrm{max}}^m(\epsilon) -\sigma_{\textrm{min}}^m(\epsilon) \textrm{d}\epsilon}{\int_{\epsilon_{\textrm{min}}}^{\epsilon_{\textrm{max}}^m}\sigma_{\textrm{max}}^m(\epsilon) -\sigma_{\textrm{min}}^m(\epsilon)\textrm{d}\epsilon},\\
S^{\sigma}(m,\epsilon,\sigma) &= (\sigma - \sigma_{\textrm{min}}^m(\epsilon))/(\sigma_{\textrm{max}}^m(\epsilon)-\sigma_{\textrm{min}}^m(\epsilon)),
\end{split}
\end{align}
where $S^{\epsilon}(m,\cdot)$ is can be thought of as a cumulative distribution function related to the conditional density $\pi_{E | M}(\cdot |m)$ for $E$ conditioned on $M$.Thus, given a standard uniform measure $\nu_{\boldsymbol{U}}\in \mathcal{P}((0,1)^3)$ with density $\pi_{\boldsymbol{U}}=\mathcal{U}(\textbf{0},\identity_3)$, our prior density is defined as a pullback by the triangular map $S^{\bx}$,
\begin{equation}
    \pi_{\bx} = (S^{\bx})^{\sharp} \pi_{\boldsymbol{U}}.
\end{equation}
Since the prior is hierarchical, sampling from it can be done sequentially. To produce samples $\{\x^i\} =\{ (m^i,\epsilon^i,\sigma^i)\}\sim \nu_{\bx}$, we pull back standard uniform samples $\x^i = S^{-1}(\boldsymbol{u}^i)\sim \nu_{\bx}$, for $\{\boldsymbol{u}^i\}\sim \mathcal{U}(0, \identity_3)$, which is explicitly written as the sequence of samples
\begin{align}\begin{split}
    m^i &\sim \mathcal{U}(0, 1/\sqrt{3}),\\
        \epsilon^i &= {(S^{\epsilon}(m^i, \cdot))}^{-1}(u^i),\; u^i \sim \mathcal{U}(0,1),\\
    \sigma^i &\sim \mathcal{U}(\sigma_{\textrm{min}}^{m^i}(\epsilon^i),\sigma_{\textrm{max}}^{m^i}(\epsilon^i)).
    \end{split}
\end{align}
To\ satisfy the absolute continuity requirements for the methods describe in \ref{sec:transportLFI}(), we work in \emph{Gaussian-whitened coordinates}, i.e. we study the inference problem based on the joint variables ($\bx, \by)$ by first transforming the parameters, which are compactly supported in $\mathcal{A}$, to be fully supported on the unbounded domain $\mathbb{R}^3$. Defining the well-known \emph{standard normal inverse cumulative distribution function} $S^{R}: (0,1) \to \mathbb{R}$ which pushes forward a standard uniform target random variable $W \sim \mathcal{U}(0,1)$ to be equal in law to a standard normal reference variable $R \sim \mathcal{N}(0,1)$, i.e. $S^{R}(W) = \sqrt{2}\textnormal{erf}^{-1}(2W -1) \sim\mathcal{N}(0,1)$~\cite{}, the composition of maps $S^{\boldsymbol{R}\boldsymbol{X}}(\x) = S^{\boldsymbol{R}} \circ S^{\bx}(\x)$, where $S^{\boldsymbol{R}}(0,1)^3 \to \mathbb{R}^3$ is the pointwise map with $S^{R}$ components, whitens samples $\{\x^i\} \sim \nu_{\bx}$, i.e. $S^{\boldsymbol{R}\boldsymbol{X}}(\x) \sim \mathcal{N}(0,\identity_3)$. We then perform our transport based variational density estimation on the variables $(S^{\boldsymbol{R}\boldsymbol{X}}(\boldsymbol{X}),\by)$. 

For density evaluations, one needs the change of variables formula

\begin{figure}
    \centering
    \caption{Visualizing the transformation:Whitened Prior samples, Uniform samples, Prior samples, Arrows, colored by a rainbow scheme.
}
    \label{fig:my_label}
\end{figure}
 As a preprocessing step, we also compute emprical cumulative distribution functions for the marginal variables $(E,\Sigma)$, since we don not have analytical forms for the  marginal densities $\pi_{E}$ and $\pi_{\Sigma}$. These emprical CDFs enable the computation of marginal inference
 
To evaluate the density of the
